# Supplementary material for: The Iris File Extension
Source: arXiv:2506.10009 ancillary file (2025-06-13)
Supplement: Supplementary file 1 [file IrisFileExtensionSpecification-1.0.pdf]

---

# **IRIS DIGITAL SLIDE FILE EXTENSION**

## **File Structure Technical Specification**

**Version 1.0**

**Copyright © 2025 Iris Developers**

**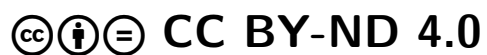 CC BY-ND 4.0**

**Prepared by Ryan Landvater**

---

# Contents

|          |                                            |          |
|----------|--------------------------------------------|----------|
| <b>1</b> | <b>Introduction</b>                        | <b>4</b> |
| 1.1      | Purpose . . . . .                          | 4        |
| 1.2      | Official Implementation Releases . . . . . | 5        |
| 1.3      | Definitions . . . . .                      | 5        |
| 1.3.1    | Terms . . . . .                            | 5        |
| 1.3.2    | Symbols and Abbreviations . . . . .        | 6        |
| 1.4      | Technical Requirements . . . . .           | 7        |
| <b>2</b> | <b>File Structure Elements</b>             | <b>9</b> |
| 2.1      | Overview . . . . .                         | 9        |
| 2.2      | Statically Defined Values . . . . .        | 9        |
| 2.2.1    | Recovery Codes . . . . .                   | 11       |
| 2.2.2    | Tile Encodings . . . . .                   | 11       |
| 2.2.3    | Pixel Formats . . . . .                    | 12       |
| 2.2.4    | Metadata Formats . . . . .                 | 12       |
| 2.2.5    | Annotation types . . . . .                 | 12       |
| 2.2.6    | Image Encoding . . . . .                   | 13       |
| 2.2.7    | Image Orientations . . . . .               | 13       |
| 2.3      | Header blocks . . . . .                    | 13       |
| 2.3.1    | File Header . . . . .                      | 14       |
| 2.3.2    | Tile Table Header . . . . .                | 17       |
| 2.3.3    | Codec Cipher . . . . .                     | 17       |
| 2.3.4    | Metadata . . . . .                         | 19       |
| 2.3.5    | Attributes . . . . .                       | 20       |
| 2.4      | Array blocks . . . . .                     | 23       |
| 2.4.1    | Layer Extents Array . . . . .              | 23       |
| 2.4.2    | Tile Offsets Array . . . . .               | 24       |
| 2.4.3    | Tile Pixel Data Array . . . . .            | 27       |
| 2.4.4    | Attribute Size Array . . . . .             | 27       |
| 2.4.5    | Attribute Byte Array . . . . .             | 29       |
| 2.4.6    | Images Array . . . . .                     | 30       |
| 2.4.7    | Images Bytes . . . . .                     | 31       |
| 2.4.8    | ICC Color Profile . . . . .                | 32       |
| 2.4.9    | Annotations Array . . . . .                | 33       |
| 2.4.10   | Annotation Byte Array . . . . .            | 35       |
| 2.4.11   | Annotation Group Sizes . . . . .           | 37       |
| 2.4.12   | Annotation Group Bytes . . . . .           | 38       |

# **Revision History**

## **VERSION 1.0 (Ratified 2025-03-27)**

### **Authors**

Ryan Landvater MD MEng, Mustafa Yousif MD, and Ulysses J Balis MD

# 1 Introduction

## 1.1 Purpose

The Iris Digital Slide file structure specification defines a portable serialization format for digital pathology whole slide image (WSI) pixel data and metadata. The Iris File Extension (IFE) structure was designed as a:

1. Highly performant binary structure amenable to:
  - a) Massively multi-threaded file encoding writes
  - b) Multi-threaded immediate random access to slide data
2. Dynamically defined file layout that:
  - a) Easily conforms to established workflows
  - b) Delegates information ordering to the encoder implementation
  - c) Allows for easily configured optional data-blocks
  - d) Allows for unobtrusive file updates
  - e) Allows for complete bi-directional file and encoder version compatibility
3. 3. Secure file format that validates structures and allows data-recovery:
  - a) That prevents file bound and buffer overflow violations
  - b) That recovers the file structure if header metadata is corrupted
4. Simplified, short, and easily readable specification

The IFE file structure has similarities to the Tagged Image File Format (TIFF) but with a performance intent and limited scope with elements that are specific to digital pathology. The byte structure is self-describing, allows fast explicit random access, is optionally zero-copy, and is influenced by modern advancements in language neutral performance serialization technology.

This specification will not describe the strengths or weaknesses of other digital slide file extensions in an effort to maintain this document as a succinct reference resource with a narrow scope. We will only define the anticipated use-case for the IFE, which is to function as an intermediate and ephemeral file format for high-speed WSI file servers and rendering of local slide files on a client machine. The IFE does not attempt to provide an alternative to the Digital Imaging and Communications in Medicine (DICOM)

standard; rather, we the authors hope it functions as a complementary high-speed exchange format within the scope of day-to-day digital pathology workflows. If interested in the historical and WSI context at the time IFE was designed, we direct the reader to the initial Iris File Extension publication with which this specification was published.

The IFE was designed by Dr. Ryan Landvater with clinical consultation from Dr. Mustafa Yousif and under the guidance of Dr. Ulysses Balis within the University of Michigan Department of Pathology. Developers of the Iris Digital Pathology system, including the IFE, are referred to as the “Iris Developers” and ratify the file extension specification until such a time as a more formalized specification committee is established.

Copyright of the Iris File Extension is owned by the Iris Developers and by the University of Michigan. Use of the IFE standard is fully available to anyone under the [Creative Commons Attribution-NoDerivatives 4.0](#) international license requiring attribution of the copyright owners and without published modification of the standard © ⓘ ⊖.

## 1.2 Official Implementation Releases

The Iris Developers support official C++ implementations with multiple language bindings, including Python and Javascript WebAssembly (WASM).

Please refer to the official [Iris Digital Pathology Github repository](#), online documentation, and license regarding incorporating these official implementations into your code base. These official implementations are licensed under MIT Software License but use may not violate the specification license that protects the IFE.

## 1.3 Definitions

### 1.3.1 Terms

The use of “**shall**” indicates a mandatory requirement within the standard. Deviation from “**shall statements**” violates the standard.

The use of “**should**” indicates an optional but suggested method for information formatting. Adhering to “**should statements**” may reduce future re-formatting for compliance, ensures non-explicitly defined requirements are intuitively defined, and follow good practice.

The use of “**may**” indicates optional implementation and/or formatting without explicit requirements. Such statements should be implemented if contextually relevant circumstances arise but use or lack thereof does not explicitly violate the standard.

The use of the term “**implementation**” or “**implementations**” shall refer to computer code, either source code or machine code, with the capacity to execute computational tasks in a way that adheres to this standard.

The use of the term “**atomic variable**” or “**atomic**” shall refer to a basic data variable that can be modified with a guarantee that no other concurrent processes (such as a thread) would see any intermediary state and without locking execution.

The use of the term “**offset pointer**” or “**offset**” shall refer to an unsigned 64-bit integer value corresponding to the number of bytes from the start of file (SOF) towards the end of file (EOF) that the first byte of a file structure element (Chapter 2) is located.

The use of the term “**slide tile**” or “**tile**” shall correspond with an array of 65,536 pixel values for a 256 x 256 pixel sub-image comprising one or more color channels in a compressed or uncompressed format.

The use of the term “**slide layer**” or “**layer**” shall correspond with a series of slide tiles that comprise a view of a whole slide image at a single defined magnification (scale). When arranged in a listed format of  $N$  length, layers shall be arranged from lowest resolution (scale), index 0, to greatest resolution (scale), index  $N - 1$ . **Note:** this layer arrangement is opposite to the layer arrangements in some contemporary API at the time of publication, such as OpenSlide. The IFE was designed from the perspective of integration with viewer systems, which will display the lowest-resolution layer first.

The use of the term “**magnification**” shall differ from the term “**scale**” in that magnification shall refer to the true microscopic optical magnification whereas scale shall refer to the relative resolution of layers to a standard base resolution. The magnification shall be related to the scale as the product of the scale with a empirically derived scaling coefficient.

The use of the term “**slide space**” or “**fractional tile location**” shall refer to a horizontal ( $X$ ) and vertical ( $Y$ ) floating point (decimal) spatial axis that can be used to define a location within a rendered slide that is layer independent. The value along an axis shall be defined as the pixel location at the lowest-resolution layer ( $l_0$ ) divided by 256 pixels to give the decimal number of lowest-resolution layer tiles such that a location or size  $(x, y)$  in **slide space** ranges from  $([0, T_{0x}], [0, T_{0y}])$  where the origin  $(0, 0)$  is defined as the upper-left of the slide and the point  $(T_{0x}, T_{0y})$  is defined as the lower-right of the slide using the same axis as the global slide indexing scheme (Figure 2.4.1), layer 0.

### 1.3.2 Symbols and Abbreviations

**DICOM** Digital Imaging and Communications in Medicine.

**EOF** end of file.

**I2S** Iris Interoperability Standard.

**ICC** International Color Consortium.

**IEC** International Electrotechnical Commission.

**IEEE** Institute of Electrical and Electronics Engineers.

**IFE** Iris File Extension.

**NEMA** National Electrical Manufacturers Association.

**SOF** start of file.

**TIFF** Tagged Image File Format.

**WASM** WebAssembly.

**WSI** whole slide image.

## 1.4 Technical Requirements

We suggest at least 64-bit architectures; though our requirements of little-endian ordering allows for native 32-bit backwards compatibility (within the numerical limits of 32-bit integers). The IFE requires all multi-byte values **shall** be stored in the little-endian byte ordering without exception. Floating point values **shall** be encoded using the Institute of Electrical and Electronics Engineers (IEEE) and International Electrotechnical Commission (IEC) established (IEEE-754/IEC-559) technical standard for floating-point arithmetic. This holds true for 16 (half-precision), 32 (single precision), and 64 (double precision) bit floating points. Metadata attributes **should** be encoded using both ASCII for key entries and UTF-8 for corresponding entry values. Alternatively, the metadata attributes **may** be encoded using the DICOM tag-value pairs and **shall** follow the corresponding required character set as established by the National Electrical Manufacturers Association (NEMA).

The official implementations provided by the Iris Developers (Section 1.2) includes convenience conversions to and from little-endian byte ordering for big-endian systems as well as convenience functions that allow conversion to and from serialized IEEE-754 floating point values. Unofficial implementations must ensure all data is serialized to these specifications.

When designed, IFE was intended to be used with atomic variables, in order to control lock-less file region access, and was intended to be used with file mapping, for random-access into tile data. This limits WASM implementations to compiling with the [Emscripten](#) SDK at the time of this document. The IFE was developed out of work on [Iris](#)

[Core](#) (the rendering module) and [Iris Codec](#) (the compression module). Consequently, the on-disk file structures mirror those defined in the Iris header files. Implementing the IFE is simplified considerably by including the freely-available [Iris headers](#) files. While the technical requirements of the file structure encoder and decoder cannot directly require including atomics, mapping, and Iris headers in an implementation, per say, these elements are critical from a pragmatic perspective in developing a clean efficient implementation. File mapping is essentially required due to the random-access lookup tile tables (which we recommend should stay in memory after being read from disk). This limits JavaScript implementations to Emscripten at the time of publication, as it is the only Web-Assembly developer kit that permits this operation in virtual file space. The use of the Iris headers and use of atomics are also strongly recommended in any implementation of this standard to successfully achieve the goals described in the *purpose* (Section [1.1](#)).



## 2 File Structure Elements

### 2.1 Overview

The file structure can be thought of as a series of floating statically defined and tightly packed data-blocks within a sea of bytes. This is due to the dynamic nature of the file format. These statically sized data-blocks, referred to as *header blocks* (Section 2.3; Figure 2.2, *horizontal hashings*), are explicitly defined structures containing data parameters, each parameter ranging from 8- to 64-bits in size that define image features or provide offsets to additional data blocks, creating an offset linkage map (also referred to as the offset-chain).

The remainder and majority of the file is made of *array blocks* (Section 2.4). These array types typically have a small header at the front for validation but are mostly composed of variable sized sequences of statically defined *entries*. In the construction of these arrays, all entries are located within a single tightly packed contiguous block without padding and contain a defined number of fixed sized (or rarely variably sized) serialized entries, with the exception of the *tile pixel data array* (Section 2.4.3). If structures are defined and the array is not simply bytes, the repeated structures are similar to header blocks in that they contain tightly packed parameters of a static size, defined at encoding time.

The overall file structure requires entry at the *file header* (Section 2.3.1), which is the statically defined first *header block* following the SOF. The dynamic file structure follows a series of linked offset values that point to other data-blocks (Figure 2.2). Each data-block, either header or array, validates its own location within the file by storing its own byte offset at the structure start followed by its recovery code identifying the data structure type (Figure 2.3). These elements will be fully described below.

### 2.2 Statically Defined Values

The following constants are defined in the specification and reserved for use in the designated contexts. These will be referenced throughout the rest of the specification. Null-type constants generally indicate an optional data-element is not present and **should** be used to indicate an unused optional parameter rather than creating a data-block with zero entries.

## Iris File Extension File Structure Outline

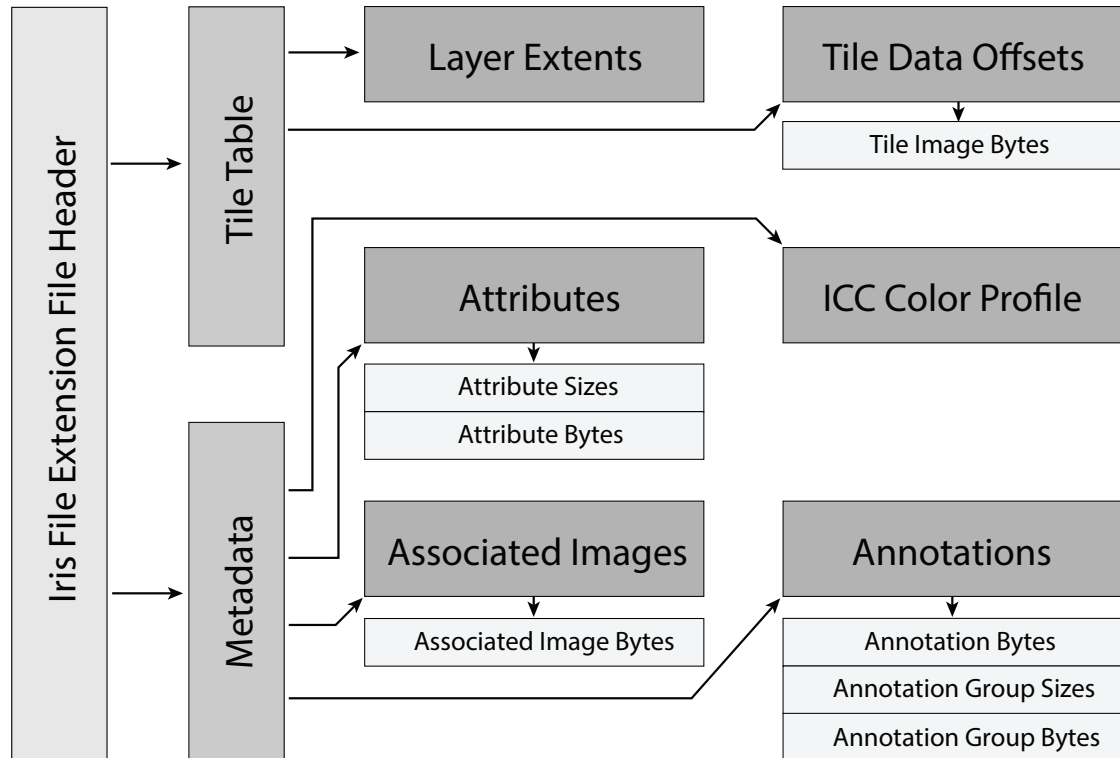

Figure 2.1: The Iris file structure follows a series of linked data blocks that extend four layers deep. More data blocks may be added in future revisions and more layers may be added to file depth if needed. The *file header* (2.3.1) points to *tile table* (2.3.2) and *metadata* (2.3.4) blocks. The *tile table* points to the *layer extents* (2.4.1) and *tile offsets* (2.4.2), which describes where to read serialized tile data. In the same layer, the *metadata* points to *attributes* (2.3.5), *associated images* (2.4.6), *ICC color profile* (2.4.8), and *annotations array* (2.4.9). Many of these tertiary data blocks are array types (Section 2.4) and point to raw byte blocks that contain serialized data (white boxes). Copyright 2025 © Iris Developers

| Parameter   | Value              | Context               |
|-------------|--------------------|-----------------------|
| NULL_OFFSET | 0xFFFFFFFFFFFFFFFF | Byte offset location  |
| MAGIC_BYTES | 0x49726973         | File Magic Bytes      |
| NULL_TILE   | 0xFFFFFFFFFFFFFFFF | Tile offset location  |
| NULL_ID     | 0xFFFFFFFFFFFFFFFF | Annotation identifier |

### 2.2.1 Recovery Codes

Recovery codes **shall** be placed after offset validation within all structures. These enumeration values **shall** be encoded as 16-bit little-endian flags. Recovery codes are used for file structure recovery in the event of corruption. The numerical recovery sequence (0...N) enumeration co-occurs with high entropy byte 0x55 as an extra precaution to further avoid spurious matches during recovery routines.

| Recovery Code                  | Value  |
|--------------------------------|--------|
| RECOVER_UNDEFINED              | 0x5500 |
| RECOVER_HEADER                 | 0x5501 |
| RECOVER_TILE_TABLE             | 0x5502 |
| RECOVER_CIPHER                 | 0x5503 |
| RECOVER_METADATA               | 0x5504 |
| RECOVER_ATTRIBUTES             | 0x5505 |
| RECOVER_LAYER_EXTENTS          | 0x5506 |
| RECOVER_TILE_OFFSETS           | 0x5507 |
| RECOVER_ATTRIBUTES_SIZES       | 0x5508 |
| RECOVER_ATTRIBUTES_BYTES       | 0x5509 |
| RECOVER_ASSOCIATED_IMAGES      | 0x550A |
| RECOVER_ASSOCIATED_IMAGE_BYTES | 0x550B |
| RECOVER_ICC_PROFILE            | 0x550C |
| RECOVER_ANNOTATIONS            | 0x550D |
| RECOVER_ANNOTATION_BYTES       | 0x550E |
| RECOVER_ANNOTATION_GROUP_SIZES | 0x550F |
| RECOVER_ANNOTATION_GROUP_BYTES | 0x5510 |

### 2.2.2 Tile Encodings

The encoding entry defines the type of byte stream used to compress the slide tile pixel values within the tile *pixel data array* (Section 2.4.3). The Iris Codec entry is currently reserved but unused.

| Encoding Algorithm      | Value | Description        |
|-------------------------|-------|--------------------|
| TILE_ENCODING_UNDEFINED | 0     | INVALID ENCODING   |
| TILE_ENCODING_IRIS      | 1     | INVALID / RESERVED |
| TILE_ENCODING_JPEG      | 2     | JPEG tiles         |
| TILE_ENCODING_AVIF      | 3     | AVIF tiles         |

### 2.2.3 Pixel Formats

The following are the supported pixel byte ordering formats. These follow the standard notation of channel followed by bits consumed by that channel. These values **should** be included as original encoding provides information about bit-depth and transparency; though **may** be excluded.

| Pixel format     | Value | Description                |
|------------------|-------|----------------------------|
| FORMAT_UNDEFINED | 0     | INVALID FORMAT             |
| FORMAT_B8G8R8    | 1     | 8-bit Blue-green-red       |
| FORMAT_R8G8B8    | 2     | 8-bit Red-green-blue       |
| FORMAT_B8G8R8A8  | 3     | 8-bit Blue-green-red-alpha |
| FORMAT_R8G8B8A8  | 4     | 8-bit Red-green-blue-alpha |

### 2.2.4 Metadata Formats

Clinical and slide acquisition metadata, among other data not directly required for slide rendering, is encoded as a series of attributes. Attributes may be encoded either according to a metadata specification known as the Iris Interoperability Standard (I2S) or directly according to the DICOM Specification Part 3 ([Information Object Definitions](#)). Optionally, metadata information can be written without adherence to a standard (METADATA\_FREE\_TEXT), but the encoding format still follows the key-value pair structure and thus uses the I2S format enumeration.

| Metadata format    | Value        | Description                    |
|--------------------|--------------|--------------------------------|
| METADATA_UNDEFINED | 0            | INVALID FORMAT                 |
| METADATA_I2S       | 1            | Iris Interoperability Standard |
| METADATA_DICOM     | 2            | <a href="#">DICOM PS3.3</a>    |
| METADATA_FREE_TEXT | METADATA_I2S | No specification               |

### 2.2.5 Annotation types

The annotation type value describes the encoding of the annotation visual object byte-stream and **shall** follow the external specifications (such as those defined for PNG or SVG).

| Annotation type      | Value | Description           |
|----------------------|-------|-----------------------|
| ANNOTATION_UNDEFINED | 0     | INVALID ANNOTATION    |
| ANNOTATION_PNG       | 1     | PNG image annotation  |
| ANNOTATION_SVG       | 2     | SVG vector annotation |
| ANNOTATION_TEXT      | 3     | Text-only annotation  |

### 2.2.6 Image Encoding

Image encoding specifically refers to associated or ancillary images and the codec used for the compression of these images. **NOTE:** This is distinct from the main WSI tile encoding algorithms, referred to as ‘Tile Encoding’ (Enumeration [2.2.2](#)).

| Annotation type          | Value | Description      |
|--------------------------|-------|------------------|
| IMAGE_ENCODING_UNDEFINED | 0     | INVALID ENCODING |
| IMAGE_ENCODING_PNG       | 1     | PNG image        |
| IMAGE_ENCODING_JPEG      | 2     | JPEG image       |
| IMAGE_ENCODING_AVIF      | 3     | AVIF image       |

### 2.2.7 Image Orientations

Image orientation is encoded as a 16-bit (half-precision) floating point but interpreted with a 360 modulo operator such that the encoded values represent intended degrees of rotation when viewing associated images such as labels or thumbnails. Common values are provided as enumerated serialized hexadecimal values below for ease.

| Annotation type       | Value  | Description                           |
|-----------------------|--------|---------------------------------------|
| ORIENTATION_0         | 0      | No rotation                           |
| ORIENTATION_90        | 0x55A0 | 90 degree clockwise rotation          |
| ORIENTATION_180       | 0x59A0 | Rotational inversion                  |
| ORIENTATION_270       | 0x5C38 | 270 degree clockwise rotation         |
| ORIENTATION_minus_90  | 0xD5A0 | 90 degree counter-clockwise rotation  |
| ORIENTATION_minus_180 | 0xD9A0 | Rotational inversion                  |
| ORIENTATION_minus_270 | 0xDC38 | 270 degree counter-clockwise rotation |

## 2.3 Header blocks

All data within header blocks **shall** be tightly packed with explicitly defined offset locations for each parameter within the header structure. The location of any header block within the file **may** aligned by padding if desired (word, page, etc); however there is no explicit need to do so nor benefit of doing so. Regardless of the contents of header blocks, there **should** be two (2) required parameters, the offset validation and the recovery code:

| Parameter                 | Type               | Offset |
|---------------------------|--------------------|--------|
| Offset validation         | 64-bit unsigned    | 0      |
| Recovery code             | 16-bit enumeration | 8      |
| Any additional parameters | ...                | 10     |
| Final / Static Size       |                    | size   |

The only exception is the *file header* (Section 2.3.1), which instead contains the 32-bit magic bytes instead of the offset location.

The remainder of this section will detail each statically-sized header block. Section 2.4 will then cover the array blocks.

### 2.3.1 File Header

#### Description

The file header is the only data structure with a statically defined location within the IFE. The file header provides the root entry into the file structure and contains file validation parameters such as the file magic bytes and the file size.

#### Version 1.0 Layout

| Parameter         | Type               | Offset | Value                |
|-------------------|--------------------|--------|----------------------|
| Magic Bytes       | 32-bit unsigned    | 0      | 0x49726973           |
| Recovery code     | 16-bit enumeration | 4      | 0x5501               |
| File Size         | 64-bit unsigned    | 6      | file size in bytes   |
| ISE Major Version | 16-bit unsigned    | 14     | 0x0001               |
| ISE Minor Version | 16-bit unsigned    | 16     | 0x0000               |
| File Revision     | 32-bit unsigned    | 18     | file revision number |
| Tile Table Offset | 64-bit offset      | 22     | Section 2.3.2        |
| Metadata Offset   | 64-bit offset      | 30     | Section 2.3.4        |
| Size              |                    | 38     |                      |

#### Specification

The overall size of the IFE v1.0 file header is **38 bytes**. The first byte of the file **shall** also be the first byte of the file header. Iris file extension's Magic Bytes are ASCII for 'Iris' (0x49726973) and **shall** be encoded in little-endian ordering. The file size **shall** be encoded as a 64-bit unsigned integer identical to the operating system query for the file size in bytes. The Iris extension version (IFE version) **shall** contain this specification version in the form of two 16-bit unsigned integers with the ISE major version followed by the the ISE minor version. The file revision number is an incremented file counter that **shall** be incremented each time a file modification has occurred. The tile table offset **shall** contain a valid file offset location to the tile table header (defined in subsection 2.3.2). The metadata header offset **shall** contain a valid offset location of the metadata header (defined in subsection 2.3.4).

## Examples of Iris File Extension WSI File Structures

### Our Recommended File Structure Encoding:

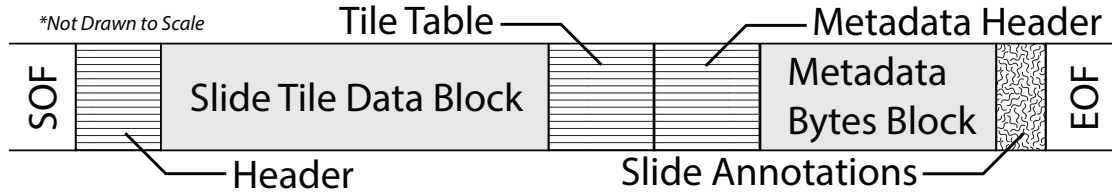

### Examples of Other Completely Valid Structures:

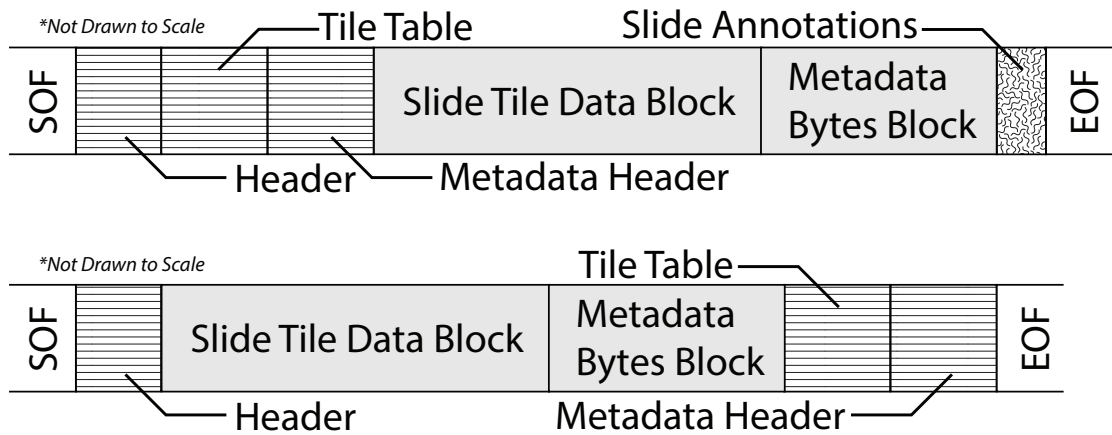

Figure 2.2: Examples of IFE allowable WSI file structures. The header blocks (horizontal hashings) include the *tile table* (Section 2.3.2, which defines the layout of tile slide tile data block shown in fig. 2.4), the *metadata header* (Section 2.3.4, which describes the layout of the raw metadata bytes / attribute concatenated string block 2.4.5), and optional slide annotations array can be placed anywhere within the file. The only static requirement is that the *file header* (Section 2.3.1) must be the first entry after the SOF. The Iris Developers recommend placing more dynamic elements such as annotations or metadata strings close to the EOF for unobtrusive file updates. Copyright 2025 © Iris Developers

## Iris File Extension Offset and Validation Schema

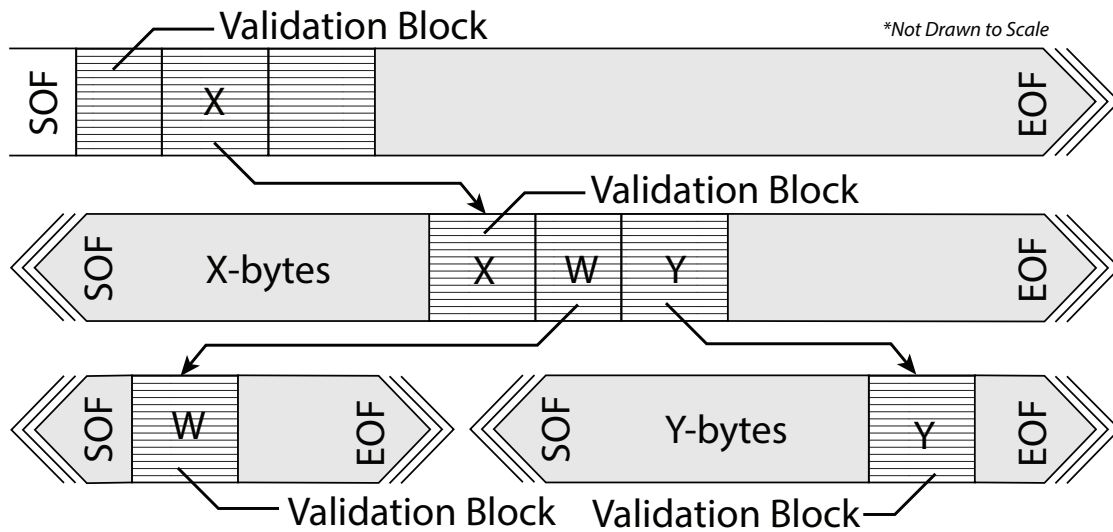

Figure 2.3: File offset linkage structure and validation schema. Iris data-blocks are dynamically situated at encoder defined 64-bit unsigned byte offset locations (horizontal hashing) within the slide file. A 64-bit validation location is encoded at the beginning of any data-block such that a de-serialize / read function  $read(x)$  at the offset byte location  $x$  evaluates as  $read(x) = x$ . In the above illustration, X is an unsigned 64-bit integer value. These offset pointers create the offset-chain such that the valid data-block found at X points to the valid data-blocks located at W- and Y-bytes into the file. Offsets can point to regions before or after the current offset. Copyright 2025 © Iris Developers



### 2.3.2 Tile Table Header

#### Description

The tile table header provides the information necessary to visually reconstruct (render) the whole slide image. This includes the visual dimensions, the number of layers, their scales and dimensions (*layer extent array*; Section 2.4.1), and the locations within the file of the compressed slide tile pixel data (*tile offsets array*; Section 2.4.2). The full relationship between this structure and the referenced structures that allow decoding is detailed in Figure 2.4.

#### Version 1.0 Layout

| Parameter     | Type               | Offset | Value                     |
|---------------|--------------------|--------|---------------------------|
| Validation    | 64-bit offset      | 0      | Tile table offset         |
| Recovery code | 16-bit enumeration | 8      | 0x5502                    |
| Encoding      | 8-bit enumeration  | 10     | Enumeration 2.2.2         |
| Format        | 8-bit enumeration  | 11     | Enumeration 2.2.3         |
| Cipher        | 64-bit offset      | 12     | Section 2.3.3             |
| Tile Offsets  | 64-bit offset      | 20     | Section 2.4.2             |
| Layer Extents | 64-bit offset      | 28     | Section 2.4.1             |
| Width         | 32-bit unsigned    | 36     | Width of slide in pixels  |
| Height        | 32-bit unsigned    | 40     | Height of slide in pixels |
| Size          |                    | 44     |                           |

#### Specification

The overall size of the IFE v1.0 tile table header is **44 bytes**. The tile encoding enumeration **shall** refer to the algorithm / specification used to compress the slide tile data and be one of the enumerated values (Enumeration 2.2.2), excluding the undefined value (0). The format **shall** describe the pixel channel ordering and bits consumed per channel per the accepted norm using one of the defined enumerated values (Enumeration 2.2.3) or **may** encode the undefined value (0). The Cipher offset **shall** contain the file offset of the Codec Cipher or NULL\_OFFSET if not encoded using ENCODING\_IRIS. The tile offsets **shall** contain a valid offset to the *tile offsets array* (Section 2.4.2) containing the byte offsets and sizes of each encoded tile. The layer extents **shall** contain a valid offset to the *layer extents array* (Section 2.4.2) containing the number of tiles and scale of each layer.

### 2.3.3 Codec Cipher

#### Description

The codec cipher is a reserved data-block for future use in the Iris Codec. For the time being, this offset **shall** be encoded with the value NULL\_OFFSET.

## Slide Tile Encoding Schema: Tile Tables and Layer Extents

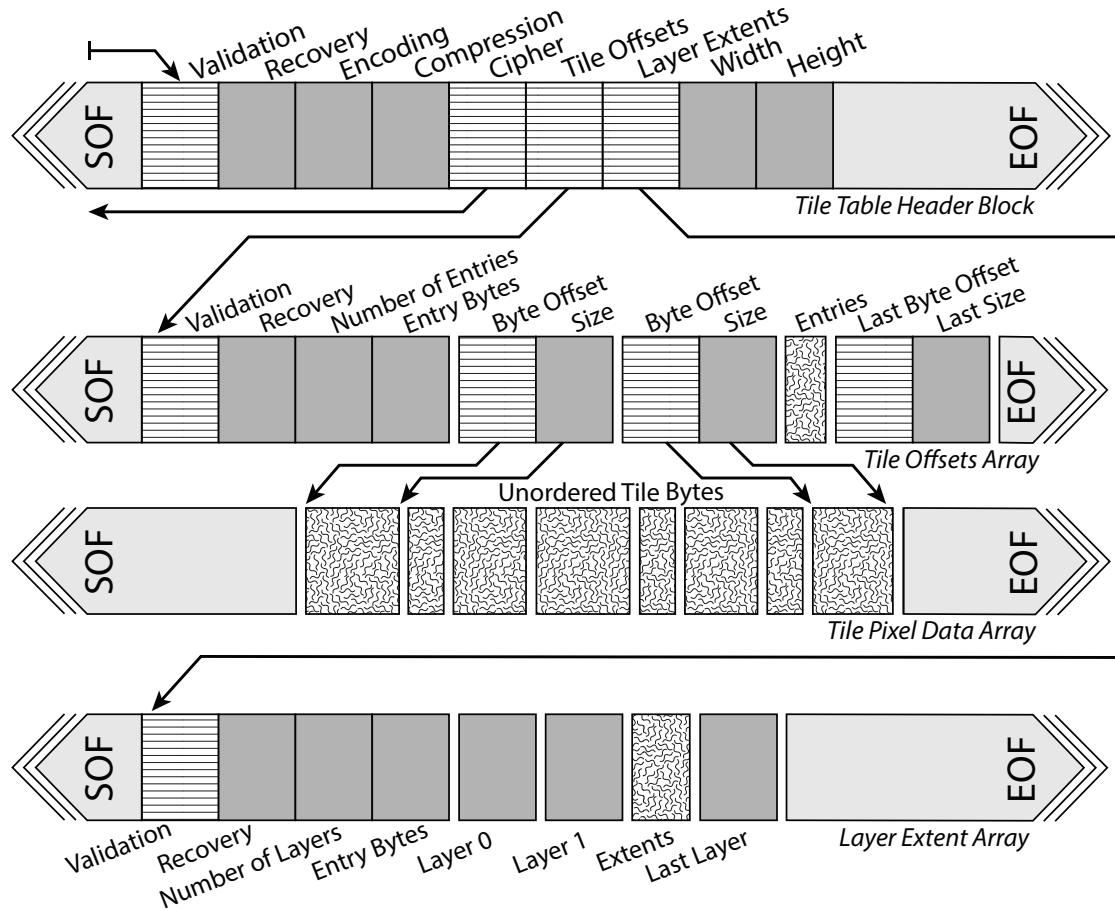

Figure 2.4: Slide tile encoding schema detailing the offset trees of the tile tables and tile arrays, and the slide / layer extents. Offset parameters are designated with horizontal hashings while value parameters are designated with gray boxes. Variable sized or a variable number of entries are designated with a texture. The *tile table* (Section 2.3.2) points to a *tile offset array* (Section 2.4.2) and a *layer extents array* (Section 2.4.1). The tile offsets array contains the offset and size in bytes of the each variably sized slide tile byte blob. The layer extent array contains parameters such as the number of tiles in each dimension and relative scale of each layer encoded in the file. Copyright 2025 © Iris Developers

### 2.3.4 Metadata

#### Description

The metadata header block provides slide metadata information, which is broken into explicitly defined slide parameters and free-form key-value pairs referred to as metadata attributes. *Attributes* (Section 2.3.5) specifically encode clinical information, and slide preparation and acquisition information. The metadata block also allows for the inclusion of labeled associated images array (Section 2.4.6), such as slide label images or thumbnail images. The ICC color space **may** be optionally encoded as an *ICC color profile* (Section 2.4.8). *Slide annotations* (Section 2.4.9) **may** also be optionally encoded within the slide file and include text, scalable vector graphics, or images, and **may** be grouped by name. Conversion coefficients **should** be included to allow for conversion between viewer zoom amounts and physical space. These values are the normalized microns per pixel ( $MpP$ ; Equation 2.1) and magnification coefficient ( $M_c$ ; Equation 2.2). The concept of microns per pixel should be familiar to programmers within the digital pathology discipline. Unlike other systems, In IFE encoded files, it **shall** be encoded normalized the slide layer with a scale of 1 – this allows for the microns per pixel to be calculated by a viewer system as the simple quotient of the  $MpP$  by the current viewer zoom scale. The  $M_c$  coefficient is similarly normalized such that the equivalent microscope objective can be calculated as the product of the  $M_c$  and current viewer zoom scale.

$$MpP = \frac{\mu m}{pixel_l} * X_l; \text{ where } X \text{ is layer scale at } l \quad (2.1)$$

$$M_c = \frac{M_l}{X_l}; \text{ where } X \text{ is layer scale at } l \quad (2.2)$$

In both equations above, layer ( $l$ ) is the is the layer where the micron distance per layer's pixel ( $pixel_l$ ) and relative magnification ( $M_l$ ) were recorded. In many implementations / slide scanners, this is this highest resolution layer. If a slide were scanned and down-sampled with layers of scale [1...64],  $X_l$  would likely be 64. This does not change / reduce the precision of the magnification and microns per pixel values; they are recorded using floating points so the location of the decimal does not affect value precision beyond floating point rounding but it does normalize these values for uniformity and to ease view system ingestion.

## Version 1.0 Layout

| Parameter         | Type                  | Offset | Value                     |
|-------------------|-----------------------|--------|---------------------------|
| Validation        | 64-bit offset         | 0      | Metadata offset           |
| Recovery code     | 16-bit enumeration    | 8      | 0x5504                    |
| Codec Major       | 16-bit unsigned       | 10     | Version if used           |
| Codec Minor       | 16-bit unsigned       | 12     | Version if used           |
| Codec Build       | 16-bit unsigned       | 14     | Instance build if used    |
| Attributes        | 64-bit offset         | 16     | Section 2.3.5             |
| Images            | 64-bit offset         | 24     | Section 2.4.6             |
| ICC Color Space   | 64-bit offset         | 32     | Section 2.4.8             |
| Annotations       | 64-bit offset         | 40     | Section 2.4.9             |
| Microns per Pixel | 32-bit floating point | 48     | Equation 2.1              |
| Magnification     | 32-bit floating point | 52     | Magnification coefficient |
| Size              |                       | 56     |                           |

## Specification

The overall size of the IFE v1.0 metadata header is **56 bytes**. The Iris Codec version entries **should** comprise 16-bit unsigned integers that correspond with the major, minor, and build numbers of the Iris Codec implementation that wrote the slide file; these values **may** be zero (0x0000) if an Iris Codec Module, or derived tool, did not write the slide file. Attributes **should** point to a valid *attribute header* (Section 2.3.5) or **shall** be NULL\_OFFSET if no attributes are encoded. Images **should** point to any associated images in an *images array* (Section 2.4.6) or **shall** be NULL\_OFFSET if no associated images are encoded. ICC color space **may** point to a byte array object of type *ICC color space* (Section 2.4.8) or **shall** be NULL\_OFFSET if no ICC color space is encoded. Annotations **may** point to a byte array object of type *Annotations* (Section 2.4.9) or **shall** be NULL\_OFFSET if no annotations are present. Normalized microns per pixel ( $MpP_N$ ) **should** encode a floating point coefficient that describes the number of microns ( $\mu m$ ) of physical space each pixel occupies, normalized for relative layer scale (Equation 2.1), or **may** encode a value of zero (0.f) if no value is available. Magnification **should** encode a floating point coefficient that converts layer scale to optical magnification corresponding to physical microscopes or **may** encode a value of zero (0.f) if no value is available.

### 2.3.5 Attributes

#### Description

The metadata attribute block allows for the encoding and decoding of key-value (or Tag-value) pairs containing clinical information, slide preparation, and / or acquisition information. Attributes are intended to follow an established clinical standard for the proper interoperability of slide information between institutions and vendors. All attributes **should** make a best effort to follow an interoperability standard and failure to validate

## Slide Metadata Schema: Slide Attributes

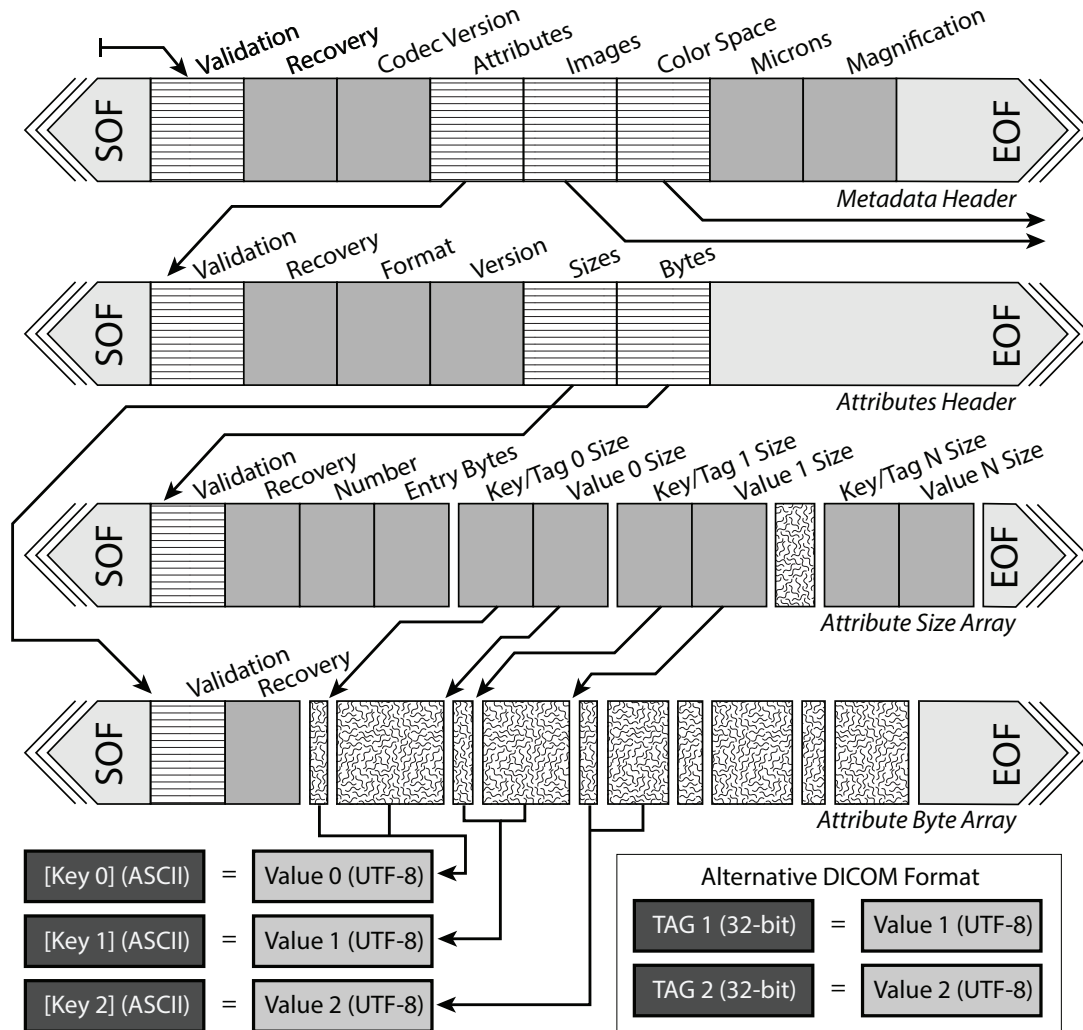

Figure 2.5: Metadata encoding schema detailing the offset trees and attribute key-value pairs. Offset parameters are designated with horizontal hashings while value parameters are designated with gray boxes. Variable sized or a variable number of entries are designated with a texture. The *metadata header block* (Section 2.3.4) points to an *attributes header* (Section 2.3.5). The attributes header contains the attributes format, specification version, if the file claims compliance, and pointers to an *attributes size array* (Section 2.4.4) and serialized *attributes bytes array* (Section 2.4.5). Attributes are de-serialized in key-value or tag-value pairs by slicing the byte array progressively by attributes size array entry. Copyright 2025 © Iris Developers

against a standard is highly discouraged. That said, the IFE provides a mechanism to encode data that does not attempt to conform to a particular standard to allow for implementations that follow established workflows that may encode unique identifiers or institutional metadata attributes (such as database keys). This may allow for avoidance of unnecessary encoding of sensitive information if present on a database for example. The metadata format for this support is METADATA\_FREE\_TEXT, which follows an encoding equivalence to that of METADATA\_I2S, and informs the decoder that the key-value pairs will follow an ASCII – UTF-8 format. Human readable data-interchange formats (or even binary object notations such as BSON) are permitted as values in the key-value pairs and may be used in rare instances if more complex structures are needed.

**NOTE:** The IFE is not intended to validate clinical interoperability metadata specification conformance; that is outside the scope of this specification.

### Version 1.0 Layout

| Parameter        | Type               | Offset | Value                         |
|------------------|--------------------|--------|-------------------------------|
| Validation       | 64-bit offset      | 0      | Metadata offset               |
| Recovery code    | 16-bit enumeration | 8      | 0x5505                        |
| Metadata Format  | 8-bit enumeration  | 10     | Section <a href="#">2.2.4</a> |
| Version          | 16-bit unsigned    | 11     | Specification version         |
| Attributes Sizes | 64-bit offset      | 13     | Section <a href="#">2.4.4</a> |
| Attributes Bytes | 64-bit offset      | 21     | Section <a href="#">2.4.5</a> |
| Size             |                    | 29     |                               |

### Specification

The overall size of the IFE v1.0 attribute header is **29 bytes**. The metadata format **shall** refer to the metadata specification format by which the file metadata was encoded and **shall** be one of the *metadata formats* (Enumeration [2.2.4](#)), excluding the undefined value (0). The version of the metadata standard (either I2S or DICOM) for which the file claims conformance **should** be encoded as a unsigned 16-bit integer in the version field. For DICOM versioning, because all [ratified changes to the standard ensure edition backwards compatibility](#) the only version information that **should** be encoded is the encoding year. If not conforming to a clinical metadata standard, the metadata format is METADATA\_FREE\_TEXT and **shall** encode the value zero (0x0000) for metadata version, to indicate the lack of claimed conformance to a standard. The attributes sizes offset **shall** encode a valid offset to the *attribute size array* (Section [2.4.4](#)), which describes how to slice the attribute byte array into pairs of key-value character strings (Figure [2.5](#)). The attributes bytes offset **shall** encode a valid offset to the *attributes byte array* (Section [2.4.5](#)), a wrapped raw byte blob containing serialized character strings.

## 2.4 Array blocks

Array blocks are similar to *header blocks* (Section 2.3) in that they are validated with the offset values encoded at their byte locations, and contain recovery codes. Unlike header blocks, which are statically sized, array blocks are *dynamically sized* and contain either 1) repeating statically sized *entries*, akin to header blocks or 2) dynamically sized byte blobs. The general outline of an array block is as follows:

| Parameter                         | Type               | Offset |
|-----------------------------------|--------------------|--------|
| Offset validation                 | 64-bit unsigned    | 0      |
| Recovery code                     | 16-bit enumeration | 8      |
| <i>Optional entry size</i>        | 32-bit unsigned    | 10     |
| <i>Optional number of entries</i> | 32-bit unsigned    | 14     |
| Array entries                     | entry              | ...    |

Often array blocks contain the size of each statically defined entry in an array of such entries (eg. Section 2.4.1) to allow for IFE version compatibility. Future versions may expand the size of a repeated element within a tightly packed array and therefore knowledge of the size of each entry at the time of encoding must be included for proper decoding alignment (despite the fact the the new content is unknown and simply treated as padding).

### 2.4.1 Layer Extents Array

#### Description

The layer extents establishes layer dimensions, which are then used for rendering and formatting of the *tile offsets array* (Section 2.4.2) formatted in accordance to the *global tile indexing scheme* (Figure 2.4.1). Layer extents must be established to unroll the multi-dimensional slide pyramidal structure into the linear global tile index values. Global index values are used for tile access within the encoding schema of the slide file. In order to convert between the 3-dimensional pyramidal and 1-dimensional linear indexing, the horizontal ( $x$ ) and vertical ( $y$ ) dimensions of each layer ( $l$ ) must be established. This array also contains scaling information (which is related to but distinct from magnification).

#### Version 1.0 Entry Layout

| Parameter  | Type                  | Offset | Value                       |
|------------|-----------------------|--------|-----------------------------|
| X-tiles    | 32-bit unsigned       | 0      | Number of tiles in $x$ -dim |
| Y-tiles    | 32-bit unsigned       | 4      | Number of tiles in $y$ -dim |
| Scale      | 32-bit floating point | 8      | Relative scale of layer     |
| Entry Size |                       | 12     |                             |

## Entry Specification

The overall size of each IFE v1.0 layer extent is **12 bytes**. The X-tiles **shall** encode the number of 256 pixel tiles in the horizontal direction and **shall** be greater than zero. The Y-tiles **shall** encode the number of 256 tiles in the vertical direction and **shall** be greater than zero. The scale  $S$  at a layer  $n$  ( $l_n$ ) **shall** encode the layer's scale  $[S(l_n)]$  as a 32-bit floating point multiple of the initial layer  $[S(l_0)]$ . The scale of a layer  $[S(l_n)]$  **shall** have a value greater than zero (0.f) and any subsequent layer ( $l_{n+1}$ ) **shall** have a scale that is greater than the previous scale  $[S(l_{n+1}) > S(l_n)]$ .

## Version 1.0 Array Layout

| Parameter     | Type               | Offset | Value                  |
|---------------|--------------------|--------|------------------------|
| Validation    | 64-bit unsigned    | 0      | Layer extent array     |
| Recovery code | 16-bit enumeration | 8      | 0x5506                 |
| Entry size    | 16-bit unsigned    | 10     | 12 ( <i>IFE v1.0</i> ) |
| Number        | 32-bit unsigned    | 12     | $L_{Total}$            |
| $l_0$         | Layer extent       | 16     |                        |
| ...           | ...                | ...    |                        |
| $L_{total}$   | Layer extent       | ...    |                        |

## Array Specification

The overall size of the IFE v1.0 layer extent array is dynamic but **at least 28 bytes** as the number of layers **shall** be greater than zero. The entry size parameter **shall** describe the number of bytes consumed by each layer extent entry at the time of encoding. This value **shall** be used during decoding for iterating over the array of layer extents regardless of the layer extent size defined by the current specification version at the time of decoding. The number parameter **shall** encode the number of layer extent entries within the array.

### 2.4.2 Tile Offsets Array

#### Description

The tile offsets array contain tuple entries giving the byte offset pointer and byte size values of a binary blob containing the compressed slide tile data. The indexing of the tile offsets array follows the *global tile index values* (Figure 2.4.1). The global tile index values shall range from zero to the total number of tile index values  $T_{total}$  ( $0 \dots T_{total}$ ). For a slide image with  $L_{total}$  layers of  $T_x$  tiles in the horizontal dimension and  $T_y$  tiles in the vertical dimension,  $T_{total}$  is defined as:

$$T_{total} = \sum_{l=0}^{L_{total}} (T_{lx} * T_{ly}) \quad (2.3)$$



## Global Tile Indexing Scheme

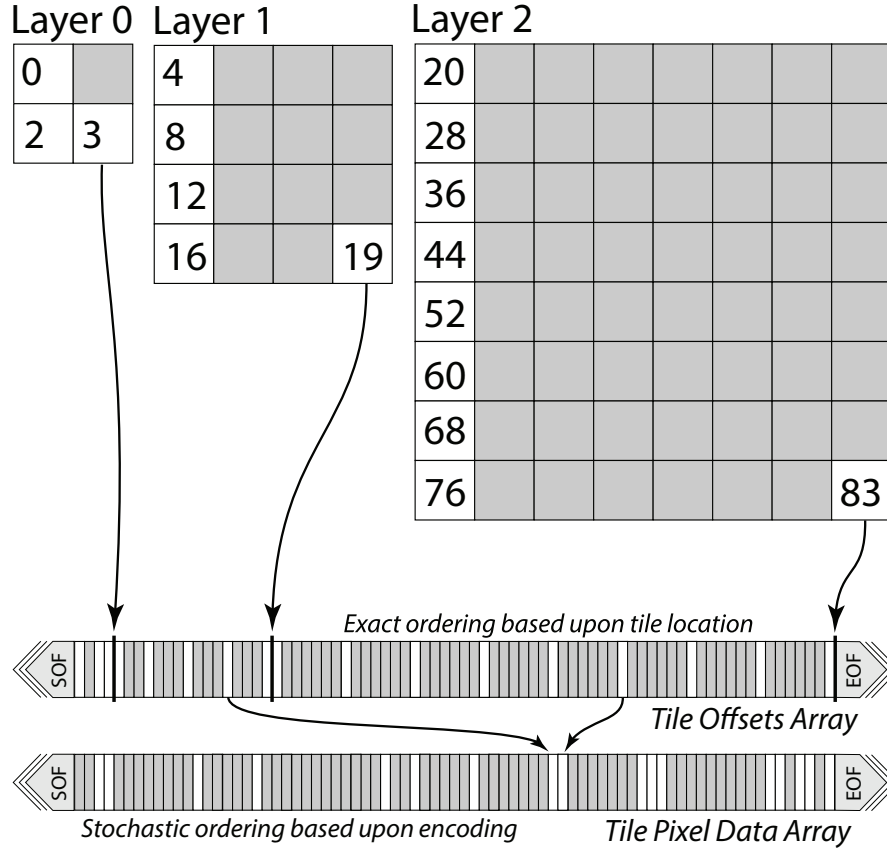

Figure 2.6: Global Tile Indexing Scheme: Tiles are packed by layer with a unique index value assigned to each tile regardless of layer. The indexing of layers is arranged from lowest scale, on the the SOF side, to highest scale towards the EOF. Tiles within layers are arranged with upper left tiles towards the SOF and bottom right towards the EOF. The total number of global indices ( $T_{total}$ ) is described in Equation 2.3. The *tile offset array* (Section 2.4.2; Figure 2.4, *second from top*) makes use of this global indexing scheme while the *tile pixel array* (Section 2.4.3; Figure 2.4, *third from top*) may not follow this ordering and rather be arranged in any order the encoder chooses, which can be entirely stochastic. Copyright 2025 © Iris Developers

The global index of a tile  $t(l, x, y)$  at location  $x$  tiles from the left and  $y$  tiles from the top at layer  $l$  within the tile offset array thus can be described as:

$$t(l, x, y) = \sum_{i=0}^{l-1} (T_{ix} * T_{iy}) + y * T_{lx} + x \quad (2.4)$$

This tile mapping scheme is described visually using numerical index value examples in Figure 2.4.1. The tile offset array structure provides rapid random-access lookup for slide tile data and is recommended by the Iris Developers that implementations retain this structure in memory after loading for optimal performance.

### Version 1.0 Entry Layout

| Parameter        | Type            | Offset | Value                   |
|------------------|-----------------|--------|-------------------------|
| Tile Data Offset | 40-bit unsigned | 0      | Location of tile data   |
| Tile Byte Size   | 24-bit unsigned | 5      | Size of data (in bytes) |
| Entry Size       |                 | 8      |                         |

### Entry Specification

The overall size of each IFE v1.0 tile offset entry is **8 bytes**. The tile byte offset **shall** encode the byte offset location relative to the SOF where the corresponding compressed tile byte-stream is located. This offset value **shall** not exceed the 40-bit max value (1.0995 terabytes) from the SOF. The tile byte size **shall** encode the number of bytes the compressed tile byte-stream consumes. The tile byte size **shall** not exceed the 24-bit max value (16.777 megabytes).

### Version 1.0 Array Layout

| Parameter     | Type               | Offset | Value                 |
|---------------|--------------------|--------|-----------------------|
| Validation    | 64-bit unsigned    | 0      | Tile offsets array    |
| Recovery code | 16-bit enumeration | 8      | 0x5507                |
| Entry size    | 16-bit unsigned    | 10     | 8 ( <i>IFE v1.0</i> ) |
| Number        | 32-bit unsigned    | 12     | $T_{total}$           |
| $t_0$         | Tile entry         | 16     |                       |
| ...           | ...                | ...    |                       |
| $T_{total}$   | Tile entry         | ...    |                       |

### Array Specification

The overall size of the IFE v1.0 tile offset array is dynamic but **at least 24 bytes** as the number of tiles **shall** be greater than zero. The entry size parameter **shall** describe the number of bytes consumed by each tile offset entry at the time of encoding. This value **shall** be used during decoding for iterating over the array of layer extents regardless of the layer extent size defined by the current specification version at the time of decoding. The number parameter **shall** encode the number of tile offset entries within the array.

### 2.4.3 Tile Pixel Data Array

#### Description

The pixel data array contains a series of raw byte blobs, each a compressed byte-stream of 65536 pixels (256 x 256 pixel tile) values according to the encoding (enumeration 2.2.2) and pixel format (enumeration 2.2.3) encoded in the *tile table header* (Section 2.3.2). Each entry is accessed via global tile index lookup (Equation 2.4) within the *tile offsets array* (Section 2.4.2) to retrieve the SOF-relative byte offset and byte-stream byte size corresponding to the requested tile index. For a visual illustration, we refer the reader to Figure 2.4, *second schematic from the bottom*.

#### Version 1.0 Entry Layout

| Parameter        | Type | Offset | Value             |
|------------------|------|--------|-------------------|
| Compressed bytes | byte | 0      | compressed stream |
| Entry Size       |      | 1      |                   |

#### Entry Specification

The compressed byte stream **shall** be comprised of one or more bytes encoded according to the encoding algorithm (enumeration 2.2.2) and pixel format (enumeration 2.2.3) encoded in the *tile table header* (Section 2.3.2).

#### Version 1.0 Array Layout

| Parameter       | Type  | Offset | Value                      |
|-----------------|-------|--------|----------------------------|
| $t_n^*$         | bytes | ...    | compressed variable length |
| $\dots^\dagger$ | ...   | ...    |                            |
| $T_{total}$     | bytes | ...    | compressed variable length |

\* the array may start with any tile index

† there is no required order to the array

#### Array Specification

The overall size of the IFE v1.0 tile pixel array is dynamic. The ordering **may** follow a global tile indexing scheme or **may** follow no indexing scheme and be arranged in any order the encoder chooses, which **may** be entirely stochastic. In addition, the array may comprise a full contiguous sequence of bytes or **may** be interrupted by intervening data.

### 2.4.4 Attribute Size Array

#### Description

The attributes size array provides the slicing information needed to convert the linear serialized *attribute byte array* (Section 2.4.5) containing  $A_{total}$  attributes into a series of

I2S key-value character string pairs or DICOM tag-value pairs, based upon the *meta-data format* (Enumeration 2.2.4) provided in the *attributes header* (Section 2.3.5) that references this array.

### Version 1.0 Entry Layout

| Parameter  | Type   | Offset | Value                |
|------------|--------|--------|----------------------|
| Key Size   | 16-bit | 0      | Key length (bytes)   |
| Value Size | 32-bit | 2      | Value length (bytes) |
| Entry Size |        | 6      |                      |

### Entry Specification

The overall size of each IFE v1.0 metadata attribute size entry **shall be 6 bytes**. The key size **shall** contain the size, in bytes, of the character string containing the attribute key. If encoded according to the DICOM standard, this value **shall** be 4 (0x0004). The value size **shall** contain the size, in bytes, of the UTF-8 formatted value byte character string containing the value corresponding to the key or tag.

### Version 1.0 Array Layout

| Parameter       | Type               | Offset | Value                 |
|-----------------|--------------------|--------|-----------------------|
| Validation      | 64-bit unsigned    | 0      | Tile offsets array    |
| Recovery code   | 16-bit enumeration | 8      | 0x5508                |
| Entry size      | 16-bit unsigned    | 10     | 6 ( <i>IFE v1.0</i> ) |
| Number          | 32-bit unsigned    | 12     | $2 * A_{total}$       |
| $A_0$           | byte               | 16     |                       |
| ...             | ...                | ...    |                       |
| $2 * A_{total}$ | byte               | ...    |                       |

### Array Specification

The overall size of the IFE v1.0 attributes size array is dynamic but **at least 16 bytes** as the number of attributes ( $A_{total}$ ) **should** be greater than zero but **may** be zero. There is no required ordering ( $A_0 \dots A_{total}$ ) for how attributes should be packed into the attributes array **except** that a key or tag shall come immediately before the corresponding value and this array **shall** follow the same ordering as the corresponding *attribute byte array* (Section 2.4.5). The entry size parameter **shall** encode the size, in bytes, of each attribute size array entry, defined above, at the time of encoding. The number parameter **shall** encode the number of sizes ( $2 * A_{total}$ ) within the array and **shall** be a integer divisible by two (2).

## 2.4.5 Attribute Byte Array

### Description

The attributes byte array contains a series of tightly packed character strings encoded as a contiguous byte block and sliced into key-value or tag-value pairs according to the series of byte sizes listed in the corresponding *attribute size array* (Section 2.4.4) and following a metadata specification defined by the format (enumeration 2.2.4) provided in the *attributes header* (Section 2.3.5) that references this array. See Figure 2.5 for a visual representation of this packing structure.

### Version 1.0 Entry Layout

| Parameter  | Type | Offset | Value                    |
|------------|------|--------|--------------------------|
| Character  | byte | 0      | ASCII or UTF-8 character |
| Entry Size |      | 1      |                          |

### Specification

The character **shall** comprise one byte of a 1-4 byte character within a serialized string. Key bytes sequences **shall** contain a string composed of ASCII Unicode or a 4-byte tag value if using the DICOM metadata specification. Value byte sequences shall contain a string composed of UTF-8 Unicode encoded free text values that correspond with the immediately preceding key or tag identifier. See Figure 2.5, *bottom pane*, for the relationship between byte array and key/tag-value pairs.

### Version 1.0 Array Layout

| Parameter     | Type               | Offset | Value                  |
|---------------|--------------------|--------|------------------------|
| Validation    | 64-bit unsigned    | 0      | Tile offsets array     |
| Recovery code | 16-bit enumeration | 8      | 0x5509                 |
| Number        | 32-bit unsigned    | 10     | Size of array in bytes |
| $C_0$         | character          | 14     |                        |
| ...           | ...                | ...    |                        |
| $C_{total}$   | character          | ...    |                        |

### Array Specification

The overall size of the IFE v1.0 attributes byte array is dynamic but **at least 14 bytes** as the number of attributes ( $A_{total}$ ) and thus characters ( $C_{total}$ ) **should** be greater than zero but **may** be zero. The number entry **shall** encode the total byte size of the attribute byte array and **shall** not exceed the 32-bit integer max value (4.29 GB).

## 2.4.6 Images Array

### Description

The images array contains  $I_{total}$  associated / ancillary images that provide additional visual information about a WSI file not a part of the WSI slide tiles. Images are referenced with unique ASCII encoded labels (eg. ‘LABEL’ or ‘THUMBNAIL’) describing the associated image. This array type allows for random access to these images by label listing and label lookup without requiring all associated images be fully loaded into memory. Like the *tile table header* (Section 2.3.2), this array has a small memory footprint, so we recommend creating an in-memory label-image dictionary once and retaining it for quick image loads (see example implementations). This array’s entries provide the parameters for each image and references a separate *image bytes* array (Section 2.4.7) for the variable-length aspects of each image, including the image label.

### Version 1.0 Entry Layout

| Parameter          | Type                  | Offset | Value                     |
|--------------------|-----------------------|--------|---------------------------|
| Image Bytes offset | 64-bit offset         | 0      | Section 2.4.7             |
| Width              | 32-bit unsigned       | 8      | Width of image in pixels  |
| Height             | 32-bit unsigned       | 12     | Height of image in pixels |
| Encoding           | 8-bit enumeration     | 16     | Enumeration 2.2.6         |
| Format             | 8-bit enumeration     | 17     | Enumeration 2.2.3         |
| Orientation        | 16-bit floating point | 18     | Enumeration 2.2.7         |
| Entry Size         |                       | 20     |                           |

### Entry Specification

The overall size of each IFE v1.0 image array entry **shall be 20 bytes**. The bytes offset **shall** encode the offset location of the variable-length image data in *image bytes* (Section 2.4.7), containing the title and compressed image byte stream. The width parameter **shall** encode the horizontal pixel extent of the encoded image and shall be greater than zero but less than the 32-bit max value. The height parameter **shall** encode the vertical pixel extent of the encoded image and **shall** be greater than zero but less than the 32-bit max value. The encoding parameter **shall** describe the compression codec used to generate the compressed image byte stream and **shall** be one of the defined enumerated values (Enumeration 2.2.6), excluding the undefined value (0). The format parameter **shall** describe the pixel channel ordering and bits consumed per channel using one of the defined enumerated values (Enumeration 2.2.3), excluding the undefined value (0). The orientation **shall** encode the intended degree of rotation for rendering the associated image as an IEEE half-precision float and **may** encode an enumerated value (Enumeration 2.2.7) but **should** encode degree value  $< 360^\circ$ .

### Version 1.0 Array layout

| Parameter     | Type               | Offset | Value                  |
|---------------|--------------------|--------|------------------------|
| Validation    | 64-bit unsigned    | 0      | Tile offsets array     |
| Recovery code | 16-bit enumeration | 8      | 0x550A                 |
| Entry size    | 16-bit unsigned    | 10     | 20 ( <i>IFE v1.0</i> ) |
| Number        | 32-bit unsigned    | 12     | $I_{total}$            |
| $I_0$         | byte               | 16     |                        |
| ...           | ...                | ...    |                        |
| $I_{total}$   | byte               | ...    |                        |

### Array Specification

The overall size of the IFE v1.0 image array is dynamic but **at least 16 bytes** as the number of bytes **should** be greater than zero but **may** be zero. There is no required ordering ( $I_0 \dots I_{total}$ ) for how images should be packed into the array. The entry size parameter **shall** encode the size, in bytes, of the image array entry (Entry Size), defined above, at the time of encoding. The number parameter shall encode the number of images  $I_{total}$  within the image array.

### 2.4.7 Images Bytes

#### Description

Image bytes contain the variable-length attributes of associated images including the unicode encoded image title / image label and the image byte-stream, compressed according to a valid *image encoding* (Enumeration 2.2.6) codec within this image's corresponding image entry within the *images array* (Section 2.4.6). These byte values are tightly packed as part of this array's dynamic region, and are sliced according to the 'Title size' and 'Image size' byte size values encoded in the header. The overall byte size of the dynamic region can be computed as the sum of the 'Title size' and 'Image size' values.

### Version 1.0 Entry Layout

| Parameter  | Type | Offset | Value                   |
|------------|------|--------|-------------------------|
| Bytes      | byte | 0      | Unicode and image bytes |
| Entry Size |      | 1      |                         |

### Entry Specification

The byte **shall** comprise one byte of a valid unicode or compressed image byte stream. If the byte contributes to an image label, the value **shall** be a valid ASCII Unicode entry, less than the 16-bit max from the start of the unicode sequence, and **shall** precede any compressed image bytes. If the byte contributes to an image byte stream, it **shall** less than the 32-bit max value bytes from the start of the image byte stream start and

**shall** contribute to image data encoded in one of the valid *image encoding* formats (Enumeration [2.2.6](#)).

#### Version 1.0 Array Layout

| Parameter     | Type               | Offset | Value              |
|---------------|--------------------|--------|--------------------|
| Validation    | 64-bit unsigned    | 0      | Tile offsets array |
| Recovery code | 16-bit enumeration | 8      | 0x550B             |
| Title Size    | 16-bit unsigned    | 10     | ASCII label bytes  |
| Image Size    | 32-bit unsigned    | 12     | Image bytes        |
| start         | byte               | 16     |                    |
| ...           | ...                | ...    |                    |
| total bytes   | byte               | ...    |                    |

#### Array Specification

The overall size of the IFE v1.0 image bytes entry is dynamic but **shall comprise more than 16 bytes** as the tile and image sizes **shall** be greater than zero. The title size **shall** encode a size, in bytes, greater than zero but shorter in length than the 16-bit max of a valid and unique image title / label. The image size **shall** encode a size, in bytes, greater than zero bytes but less than the 32-bit max (4.29 GB) of a valid encoded image byte stream encoded according to one of the valid *image encoding* formats (Enumeration [2.2.6](#)).

### 2.4.8 ICC Color Profile

#### Description

ICC profile is an optional set of data that characterizes a color input or output device, or a color space, according to standards established by the International Color Consortium (ICC). We refer the reader to the [ICC specifications](#) for more details. The ICC color profile array structure is a serialized byte buffer containing the contents of an ICC (.icc) profile without modification.

#### Version 1.0 Entry Layout

| Parameter  | Type | Offset | Value            |
|------------|------|--------|------------------|
| ICC Bytes  | byte | 0      | ICC profile byte |
| Entry Size |      | 1      |                  |

#### Entry Specification

The ICC bytes **shall** comprise one or more bytes containing a valid ICC color profile.



## Version 1.0 Array Layout

| Parameter     | Type               | Offset | Value              |
|---------------|--------------------|--------|--------------------|
| Validation    | 64-bit unsigned    | 0      | Tile offsets array |
| Recovery code | 16-bit enumeration | 8      | 0x550C             |
| Number        | 32-bit unsigned    | 10     | total bytes        |
| start         | byte               | 14     |                    |
| ...           | ...                | ...    |                    |
| end           | byte               | ...    |                    |

## Array Specification

The overall size of the IFE v1.0 ICC color profile is dynamic but **greater than 14 bytes** as the number of bytes **shall** be greater than zero. The number parameter shall encode the size of the array containing the raw ICC profile in number of bytes.

### 2.4.9 Annotations Array

#### Description

Slide annotations digitally replicate the conventional markups made to glass slides. Multiple types of annotation are permitted within the IFE. Text is included for optimal readability while vector graphics can store geometric shapes or act like images, another supported modality, to imitate traditional dotting pen annotations. Annotations are stored in a way such that they may be easily rasterized and then may be applied to the slide by a viewer system. The annotation object is intended to be decoded or rasterized to an image that matches the encoded pixel width and pixel height values, and then applied to the slide independent of these decoded dimensions – and instead sized and positioned using the floating point X and Y location and size values. Location and size values are encoded at *fractional tile locations* (definitions Section 1.3) within the *slide space* convention.

The origin of *slide space* uses the same axis as the *global tile indexing schema* (Figure 2.4.1), layer 0, which was designed to match modern graphical API such as Vulkan’s draw space convention, for programmer ease. For example, an annotation located along the x-axis 384 pixels from the far-left of the slide and measuring 128 pixels when fully zoomed out ( $l_o$ ) would be encoded with a X-location of 1.5 and a X-size of 0.5 (See Figure 1.3.1 for a visual example of fractional tile locations within the slide space convention).

Annotation groups provide a convenient mechanism for associating annotation objects of a similar type or use-case into a set that can be manipulated by viewer systems and (semi-)supervised artificial intelligence frameworks. The *group sizes* (Section 2.4.11) and *group bytes* (Section 2.4.12) arrays provide this information by in a similar structure to the attributes serialization routines, and the reader will note similarities in the byte structure and slicing mechanisms employed.

### Version 1.0 Entry Layout

| Parameter    | Type                  | Offset | Value                             |
|--------------|-----------------------|--------|-----------------------------------|
| Identifier   | 24-bit unsigned       | 0      | Annotation Identifier tag         |
| Bytes offset | 64-bit offset         | 3      | Section <a href="#">2.4.10</a>    |
| Format       | 8-bit enumeration     | 11     | Enumeration <a href="#">2.2.5</a> |
| X-location   | 32-bit floating point | 12     | Horizontal offset location        |
| Y-location   | 32-bit floating point | 16     | Vertical offset location          |
| X-size       | 32-bit floating point | 20     | Width of annotation               |
| Y-size       | 32-bit floating point | 24     | Height of annotation              |
| Pixel width  | 32-bit unsigned       | 28     | Pixel height                      |
| Pixel height | 32-bit unsigned       | 32     | Pixel width                       |
| Parent ID    | 24-bit unsigned       | 36     | Optional parent identifier        |
| Entry Size   |                       | 39     |                                   |

### Entry Specification

The overall size of each IFE v1.0 annotation entry **shall be 39 bytes**. The identifier **shall** encode a 24-bit value tag used to uniquely identify the annotation and **shall** not be the `NULL_ID` value. The bytes offset **shall** be a valid offset location that point to the corresponding attribute object's *attributes bytes array* (Section [2.4.5](#)) containing the visual object byte-stream. The format enumeration **shall** describe the byte format of the object byte stream and **shall** be one of the enumerated values (Enumeration [2.2.5](#)), excluding the undefined entry (0). The X-location and Y-location **shall** encode the *fractional tile location* of the annotation visual object origin (upper-left point) in *slide space* (Section [1.3](#)) format. The X-size and Y-size **shall** encode the size of the rendered annotation visual object in *slide space* (Terms [1.3.1](#)). The pixel width and pixel height parameters **shall** encode the image dimensions of the decoded or rasterized annotation visual object in the horizontal and vertical dimensions, respectively, and **shall** be greater than 0 but less than the max 32-bit unsigned value. The parent identifier entry **may** encode an optional parent annotation object identifier with which to link the present object and **shall** be a valid annotation identifier if used, else it **should** encode the value `NULL_ID` to indicate no parent annotation is referenced.

### Version 1.0 Array Layout

| Parameter          | Type               | Offset | Value                          |
|--------------------|--------------------|--------|--------------------------------|
| Validation         | 64-bit unsigned    | 0      | Tile offsets array             |
| Recovery code      | 16-bit enumeration | 8      | 0x550D                         |
| Entry size         | 16-bit unsigned    | 10     | 39 ( <i>IFE v1.0</i> )         |
| Number             | 32-bit unsigned    | 12     | $A_{total}$                    |
| Group Sizes Offset | 64-bit unsigned    | 16     | Section <a href="#">2.4.11</a> |
| Group Bytes Offset | 64-bit unsigned    | 24     | Section <a href="#">2.4.12</a> |
| $A_0$              | byte               | 32     |                                |
| ...                | ...                | ...    |                                |
| $A_{total}$        | byte               | ...    |                                |

### Array Specification

The overall size of the IFE v1.0 annotation array is dynamic but **at least 32 bytes** as the number of annotations **should** be greater than zero but **may** be zero. The entry size parameter shall encode the size of each annotation array entry, in bytes, at the time of encoding. The number parameter **shall** encode the number of annotations encoded and **shall** be less than the 32-bit max value.

### 2.4.10 Annotation Byte Array

#### Description

The attributes byte array provides a validation and recovery wrapper around a byte array containing the raw annotation byte stream. The annotation byte stream encodes visual annotation objects according to one of the enumerated *annotation types* (Enumeration [2.2.5](#)).

### Version 1.0 Array Layout

| Parameter       | Type | Offset | Value       |
|-----------------|------|--------|-------------|
| Annotation byte | byte | 0      | byte stream |
| Entry Size      |      | 1      |             |

### Entry Specification

The annotation byte **shall** comprise one byte of a valid visual annotation byte array in either the serialized image byte format (for image bytes) or unicode character format for text or markup style vector graphic. The byte **shall** be less than 32-bit max value from the start of the byte array sequence.

## Slide Space / Fractional Tile Locations

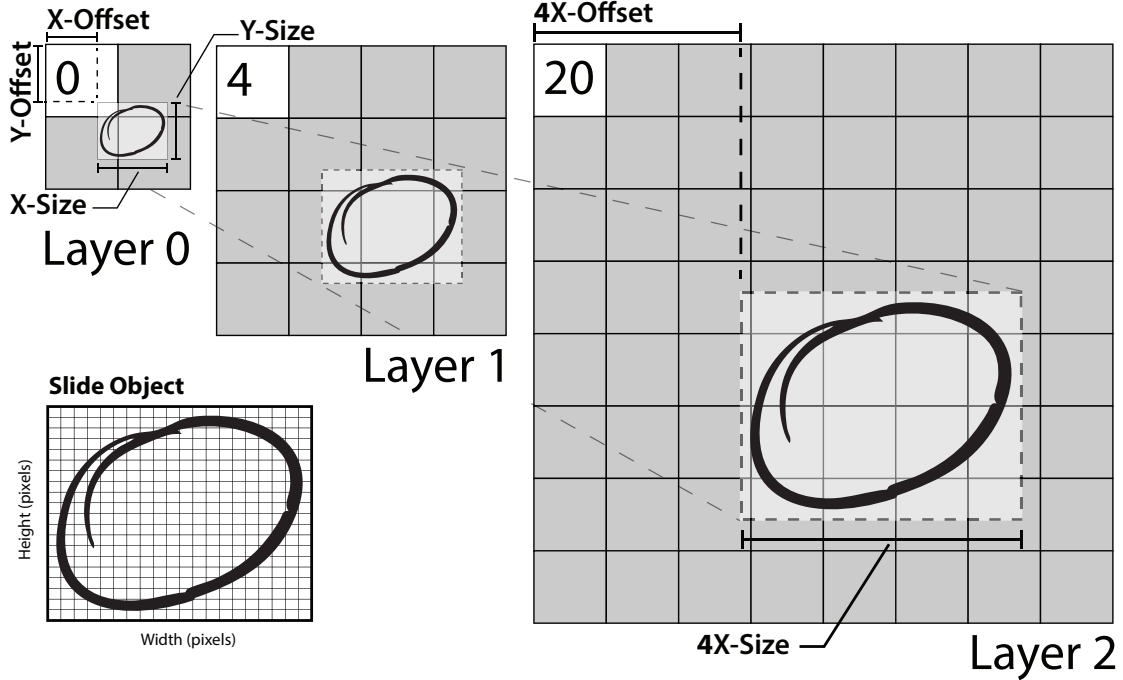

Figure 2.7: Slide objects are graphical figures, in the form of a raster graphic (that may optionally be derived from vector graphics) with the height and width dimensions in pixels (bottom-left). The rendered dimensions are separate from the raster dimensions, as they must be mapped to *slide space* (Section 1.3). The slide space is defined in fractional tile locations ranging from the upper-left slide origin  $(0.0, 0.0)$  to the full slide-layer extent at the initial layer  $(l_0)$  and can be represented as  $(T_{0x}, T_{0y})$ . The location is represented in a decimal number of 256 pixel tiles offset from the origin in the horizontal and vertical axes, respectively, and the object origin  $(O_0)$  can be expressed as a coordinate within the range of  $l_0$  tiles  $O_0 = ([0.0, T_{0x}], [0.0, T_{0y}])$ . Similarly, the drawn dimensions of the slide are represented in terms of a decimal number of tiles at layer 0 such that X- and Y-size fall within the ranges  $(0.0, T_{0x}]$  and  $(0.0, T_{0y}]$ , respectively. In the above implementation, the X-offset is approximately 0.73 tiles with an X-size of approximately 1.0 tiles. When drawn by a slide rendering implementation, such a structure can be appropriately scaled (right).

### Version 1.0 Array Layout

| Parameter     | Type               | Offset | Value                  |
|---------------|--------------------|--------|------------------------|
| Validation    | 64-bit unsigned    | 0      | Tile offsets array     |
| Recovery code | 16-bit enumeration | 8      | 0x550E                 |
| Number        | 32-bit unsigned    | 10     | Size of array in bytes |
| $B_0$         | character          | 14     |                        |
| ...           | ...                | ...    |                        |
| $B_{total}$   | character          | ...    |                        |

### Array Specification

The overall size of the IFE v1.0 annotation byte array is dynamic but **at least 14 bytes** as the number of annotation bytes ( $B_{total}$ ) **should** be greater than zero but **may** be zero. The number entry **shall** encode the total byte size of the annotation byte array and **shall** not exceed the 32-bit integer max value (4.29 GB).

### 2.4.11 Annotation Group Sizes

#### Description

The annotation group sizes data-block allows for the decoding of group-title and annotation identifier lists by providing tuples containing the title size and number of annotation identifiers associated with the aforementioned title. This array must follow the same ordering as the corresponding *annotation group bytes* array (Section [2.4.12](#))

### Version 1.0 Array Layout

| Parameter  | Type   | Offset | Value                    |
|------------|--------|--------|--------------------------|
| Title Size | 16-bit | 0      | Length (bytes)           |
| Number     | 32-bit | 2      | Number of Annotation IDs |
| Entry Size |        | 6      |                          |

### Entry Specification

The overall size of each IFE v1.0 annotation group size entry **shall be 6 bytes**. The title size **shall** contain the size, in bytes, of the character string containing the annotation group title. The number parameter **shall** contain the number of 24-bit annotation identifiers within the annotation group.

### Version 1.0 Array Layout

| Parameter     | Type               | Offset | Value                 |
|---------------|--------------------|--------|-----------------------|
| Validation    | 64-bit unsigned    | 0      | Tile offsets array    |
| Recovery code | 16-bit enumeration | 8      | 0x550F                |
| Entry size    | 16-bit unsigned    | 10     | 6 ( <i>IFE v1.0</i> ) |
| Number        | 32-bit unsigned    | 12     | $G_{total}$           |
| $G_0$         | group size entry   | 16     |                       |
| ...           | ...                | ...    |                       |
| $G_{total}$   | group size entry   | ...    |                       |

### Array Specification

The overall size of the IFE v1.0 annotation group size array is dynamic but **at least 16 bytes** as the number of annotation groups ( $G_{total}$ ) **should** be greater than zero but **may** be zero. There is no required ordering ( $G_0 \dots G_{total}$ ) for how annotation groups should be packed into the attributes array **except** that a title shall come immediately before the corresponding sequence of annotation identifiers and this array **shall** follow the same ordering as the corresponding *annotation group bytes* array (Section 2.4.12). The entry size parameter **shall** encode the size, in bytes, of each annotation group size array entry, defined above, at the time of encoding. The number parameter **shall** encode the number of annotation groups ( $G_{total}$ ) within the array.

### 2.4.12 Annotation Group Bytes

#### Description

The annotation group bytes array contains a series of tightly packed label character strings and 24-bit annotation identifier tag array encoded as a contiguous byte block and sliced into label and identifier-array pairs according to the series of sizes listed in the previously described and corresponding *annotation group sizes array* (Section 2.4.11). This slicing paradigm is similar to that employed in the attributes sizes and bytes arrays and we refer the reader to that section and corresponding figure illustration for more detailed information.

### Version 1.0 Entry Layout

| Parameter     | Type            | Offset | Value                        |
|---------------|-----------------|--------|------------------------------|
| Character     | byte            | 0      | ASCII label character        |
| Annotation ID | 24-bit unsigned | 0      | Member annotation identifier |
| Entry Size    |                 | 1 or 3 |                              |

### Specification

Each entry **shall** comprise 1 or 3 bytes corresponding with either a ASCII Unicode character or 24-bit Annotation identifier based upon sequence and location following slicing.

Label bytes sequences **shall** contain a string composed of ASCII Unicode. Annotation identifiers sequences shall contain a series of 24-bit annotation identifiers. The label character sequence shall immediately precede the annotation identifier sequence that it describes.

### Version 1.0 Array Layout

| Parameter     | Type               | Offset | Value                  |
|---------------|--------------------|--------|------------------------|
| Validation    | 64-bit unsigned    | 0      | Tile offsets array     |
| Recovery code | 16-bit enumeration | 8      | 0x5510                 |
| Number        | 32-bit unsigned    | 10     | Size of array in bytes |
| $G_0$         | Group Bytes        | 10     |                        |
| ...           | ...                | ...    |                        |
| $G_{total}$   | Group Bytes        | ...    |                        |

### Array Specification

The overall size of the IFE v1.0 annotation group bytes array is dynamic but **at least 10 bytes** as the number of groups ( $G_{total}$ ) and thus labels characters ( $C_{total}$ ) and annotation identifiers ( $A_{total}$ ) **should** be greater than zero but **may** be zero. The number entry **shall** encode the total byte size of the annotation groups bytes array and **shall** not exceed the 32-bit integer max value (4.29 GB). The number entry *bytes* **shall** be equivalent to the anticipated array size defined as the sum of *annotation group bytes* (Section 2.4.12) entries. This number entry in bytes ( $N_{total}$ ) in bytes is the sum of all annotation groups ( $G_{total}$ ). Each group is a sum of total label character bytes ( $C$ ) and number of 24-bit identifier tags ( $A$ ) according to the following expression:

$$N_{total} = \sum_{g=0}^{G_{total}} C_g + 3A_g \quad (2.5)$$
